# Supplementary material for: The negative thermal expansion mechanism of zirconium tungstate, ZrW2O8
Source: arXiv:1510.00361 source file (2016-02-16)
Supplement: Supplementary file 1 [file SupplementalInformation.pdf]

# Supplemental Material

| | DFT Calculation (This Study) | | | Neutron Diffraction at 293 K * | | |
|---|---|---|---|---|---|---|
| Space Group: | $P2_13$ | | | $P2_13$ | | |
| Cell Parameter: | a = 9.26705 | | | a = 9.15993(5) | | |
| Atom: | x | y | z | x | y | z |
| Zr | 0.000000 | 0.000000 | 0.000000 | 0.0003(4) | 0.0003(4) | 0.0003(4) |
| W1 | 0.342821 | 0.342821 | 0.342821 | 0.3412(3) | 0.3412(3) | 0.3412(3) |
| W2 | 0.598043 | 0.598043 | 0.598043 | 0.6008(3) | 0.6008(3) | 0.6008(3) |
| O1 | 0.20546 | 0.438327 | 0.445208 | 0.2071(3) | 0.4378(4) | 0.4470(3) |
| O2 | 0.783257 | 0.565352 | 0.554457 | 0.7876(3) | 0.5694(4) | 0.5565(3) |
| O3 | 0.489541 | 0.489541 | 0.489541 | 0.4916(5) | 0.4916(5) | 0.4916(5) |
| O4 | 0.236025 | 0.236025 | 0.236025 | 0.2336(3) | 0.2336(3) | 0.2336(3) |

Table S1: Comparison between 0 GPa equilibrium cell data for $ZrW_2O_8$ obtained in this study and experimental neutron diffraction data obtained at 293 K (reference below). Deviations from experiment are within expectations for a DFT calculation using the PBE functional.

* Reference: T. A. Mary, J. S. O. Evans, T. Vogt, and A. W. Sleight. Negative thermal expansion from 0.3 to 1050 Kelvin in $ZrW_2O_8$. Science, **272** (5258):90–92, 1996.

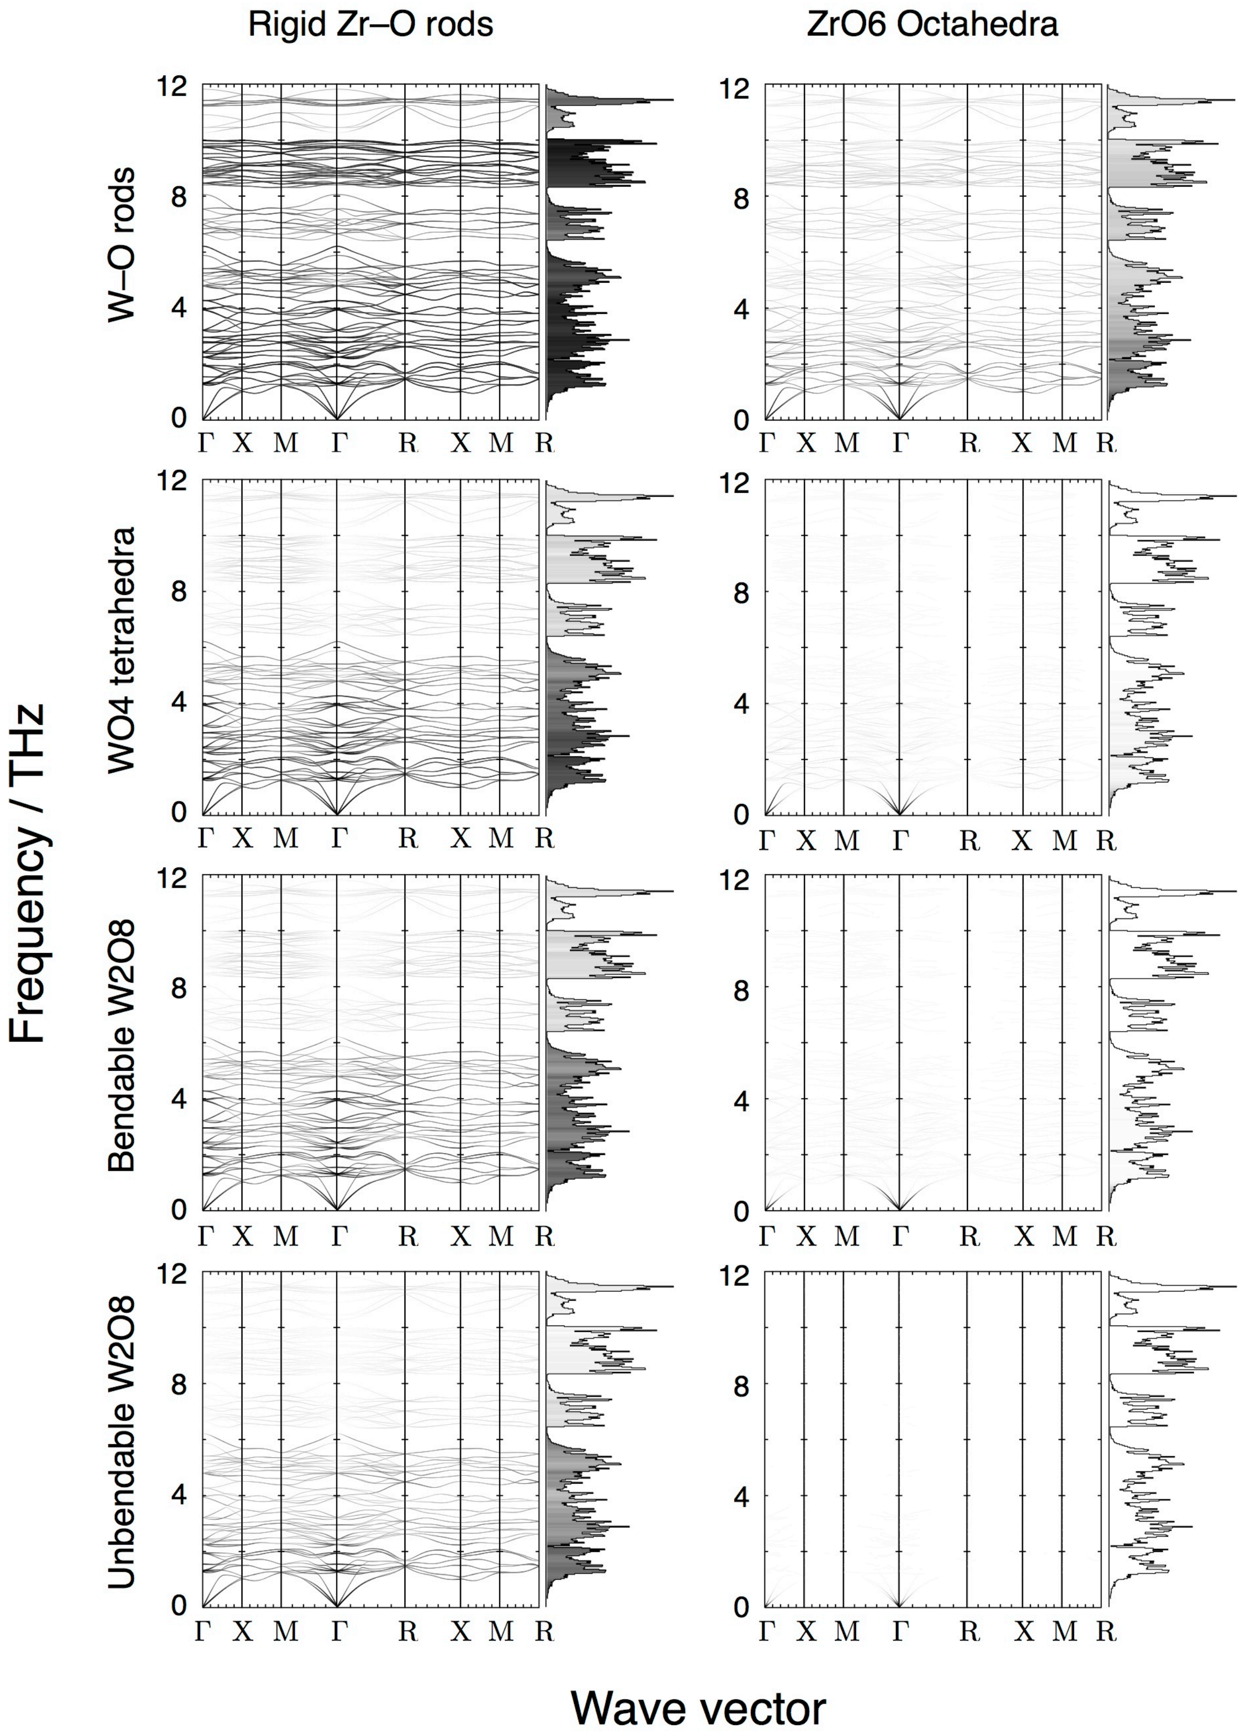


Figure S1: Flexibility analysis of $ZrW_2O_8$ phonon dispersion curves and densities of states. All data is shaded according to the value of $m_{i,k}$ at each mode for each wave vector. The shading ranges from white ($m_{i,k}$ = 0) through to black ($m_{i,k}$ = 1). Bins that make up the density of states are shaded according to the average $m_{i,k}$ for each bin using the same color scale.

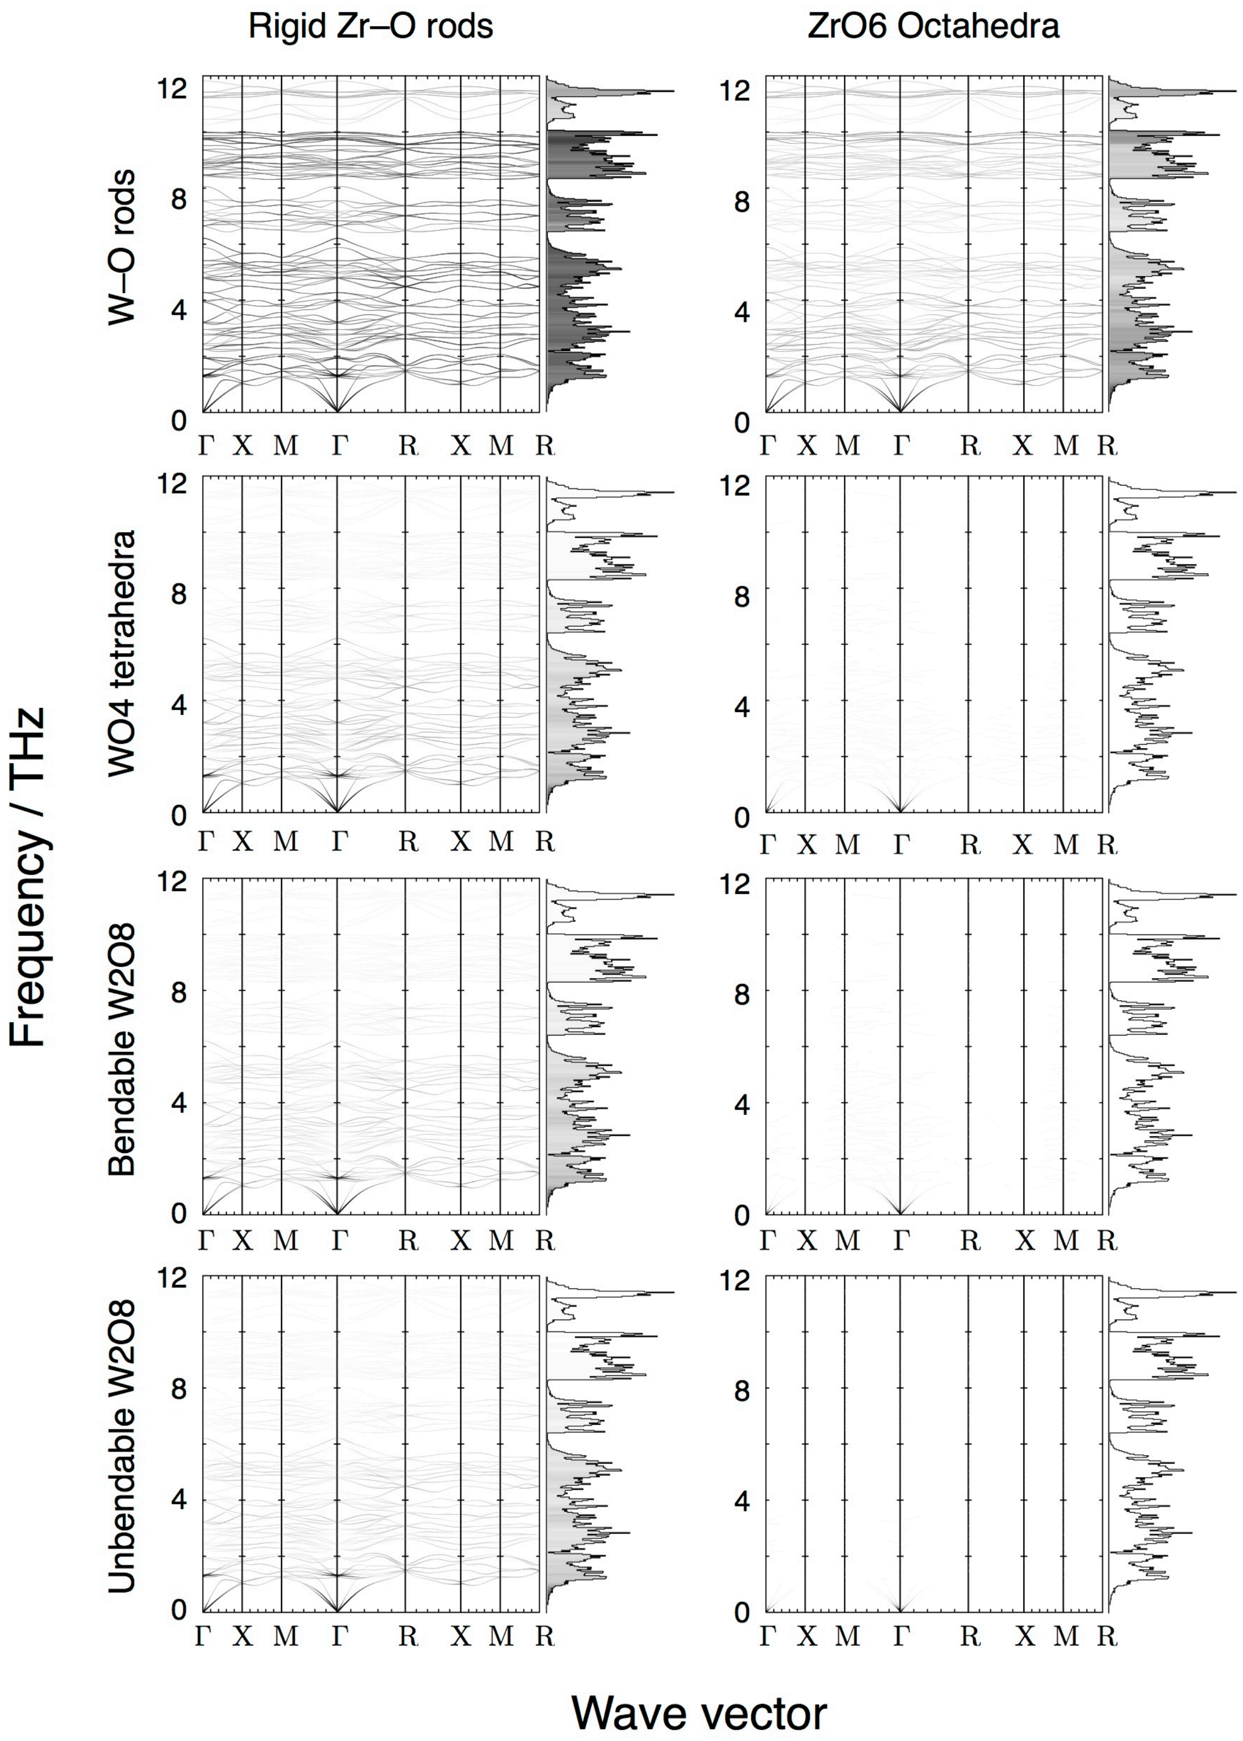


Figure S2: Further flexibility analysis of $ZrW_2O_8$ phonon dispersion curves and densities of states. All flexibility models shown here incorporate a rigid W...Zr bond. All data is shaded according to the value of mi,k at each mode for each wave vector. The shading ranges from white ($m_{i,k} = 0$) through to black ($m_{i,k} = 1$). Bins that make up the density of states are shaded according to the average $m_{i,k}$ for each bin using the same color scale.
